# Supplementary material for: Question Decomposition with Dependency Graphs
Source: arXiv:2104.08647 source file (2021-04-17)
Supplement: Supplementary file 1 [file error-analysis_bu.tex]

\onecolumn
\subsection{Error Analysis Examples}
\label{apdx:error-analysis}

Table \ref{tab:error-analysis-examples} gives some examples for the error classes from \S\ref{sec:analysis:error-analysis}.

\begin{longtable}{lll}
% {l{0.2\textwidth}l{0.4\textwidth}l{0.4\textwidth}}
\small
% \begin{tabular}{lll}
                       & Gold                                                                                                                                                                                                                                                                                                                                                                                                                                                                                                                                                                                                                                                                                                                                                                                                                                                                                                                                                                                                    & Prediction                                                                                                                                                                                                                                                                                                                                                                                                                                                                                                                                                                                                                                                                                                                                                                                                                                                                                \\ \hline
Alternative Solutions & \begin{tabular}[c]{@{}l@{}}How many   yards longer was the longest field goal over the second longest?\\      1. select(sub=field goals)\\      2. project(projection=yards of \#REF; sub=\#1)\\      3. aggregate{[}max{]}(arg=longest \#2)\\      4. aggregate{[}max{]}(arg=second longest \#2)\\      5. arithmetic{[}difference{]}(left=\#3; right=\#4)\end{tabular}                                                                                                                                                                                                                                                                                                                                                                                                                                                                                                                                                                                                                                & \begin{tabular}[c]{@{}l@{}}CopyNet\\      1. select(sub=field goals)\\      2. project(projection=yards of \#REF; sub=\#1)\\      3. aggregate{[}max{]}(arg=\#2)\\      4. discard(exclude=\#3; sub=\#2)\\      5. aggregate{[}max{]}(arg=\#4)\\      6. arithmetic{[}difference{]}(left=\#3; right=\#5)\end{tabular}                                                                                                                                                                                                                                                                                                                                                                                                                                                                                                                                                                     \\ \cline{2-3} 
                      & \begin{tabular}[c]{@{}l@{}}If there   are exactly two fluffy dogs and no reflections.\\      1. select(sub=dogs)\\      2. filter(condition=that are fluffy; sub=\#1)\\      3. aggregate{[}count{]}(arg=\#2)\\      4. boolean{[}equals\_2{]}(condition=is equal to two; sub=\#3)\\      5. select(sub=reflections)\\      6. aggregate{[}count{]}(arg=\#5)\\      7. boolean{[}equals\_0{]}(condition=is equal to zero; sub=\#6)\\      8. boolean{[}logical\_and,true{]}(sub=\#4,\#7)\end{tabular}                                                                                                                                                                                                                                                                                                                                                                                                                                                                                                   & \begin{tabular}[c]{@{}l@{}}Latent-RAT\\      1. select(sub=dogs)\\      2. filter(condition=that are fluffy; sub=\#1)\\      3. aggregate{[}count{]}(arg=\#2)\\      4. boolean{[}equals\_2{]}(condition=is equal to two; sub=\#3)\\      5. project(projection=reflections of \#REF; sub=\#2)\\      6. aggregate{[}count{]}(arg=\#5)\\      7. boolean{[}equals\_0{]}(condition=is equal to zero; sub=\#6)\\      8. boolean{[}logical\_and,true{]}(sub=\#4,\#7)\end{tabular}                                                                                                                                                                                                                                                                                                                                                                                                           \\ \hline
Elaboration Level     & \begin{tabular}[c]{@{}l@{}}What tv   program with more than 19 episodes did Joey Lawrence play on?\\      1. select(sub=Joey Lawrence)\\      2. project(projection=tv programs of \#REF; sub=\#1)\\      3. filter(condition=with more than 19 episodes; sub=\#2)\end{tabular}                                                                                                                                                                                                                                                                                                                                                                                                                                                                                                                                                                                                                                                                                                                         & \begin{tabular}[c]{@{}l@{}}BiaffineGP\\      1. select(sub=Joey Lawrence)\\      2. project(projection=tv program; sub=\#1)\\      3. project(projection=episodes; sub=\#2)\\      4. group{[}count{]}(key=\#2; value=\#3)\\      5. comparative{[}more{]}(attribute=\#4; condition=more than 19; sub=\#2)\end{tabular}                                                                                                                                                                                                                                                                                                                                                                                                                                                                                                                                                                   \\ \hline
Redundancy            & \begin{tabular}[c]{@{}l@{}}How many   TD passes were under 10 yards?\\      1. select(sub=TD passes)\\      2. project(projection=yards of \#REF; sub=\#1)\\      3. comparative{[}less{]}(attribute=\#2; condition=is lower than 10 yards;   sub=\#1)\\      4. aggregate{[}count{]}(arg=\#3)\end{tabular}                                                                                                                                                                                                                                                                                                                                                                                                                                                                                                                                                                                                                                                                                             & \begin{tabular}[c]{@{}l@{}}CopyNet\\      1. select(sub=TD passes)\\      2. project(projection=yards of \#REF; sub=\#1)\\      3. comparative{[}less{]}(attribute=\#2; condition=is lower than 10;   sub=\#1)\\      4. aggregate{[}count{]}(arg=\#3)\end{tabular}                                                                                                                                                                                                                                                                                                                                                                                                                                                                                                                                                                                                                       \\ \hline
Wrong Gold            & \begin{tabular}[c]{@{}l@{}}How many   objects are either yellow or shiny? \\      1. select(sub=objects)\\      2. filter(condition=that are yellow; sub=\#1)\\      3. filter(condition=that are shiny; sub=\#1)\\      4. aggregate{[}count{]}(arg=\#2)\\      5. aggregate{[}count{]}(arg=\#3)\\      6. arithmetic{[}sum{]}(arg=\#4,\#5)\end{tabular}                                                                                                                                                                                                                                                                                                                                                                                                                                                                                                                                                                                                                                               & \begin{tabular}[c]{@{}l@{}}BiaffineGP\\      1. select(sub=objects)\\      2. filter(condition=shiny; sub=\#1)\\      3. discard(exclude=\#2; sub=\#1)\\      4. aggregate{[}count{]}(arg=\#2)\\      5. filter(condition=yellow; sub=\#3)\\      6. aggregate{[}count{]}(arg=\#5)\\      7. arithmetic{[}sum{]}(arg=\#4,\#6)\end{tabular}                                                                                                                                                                                                                                                                                                                                                                                                                                                                                                                                                \\ \hline
Missing Information   & \begin{tabular}[c]{@{}l@{}}What shape   of the only object that wont roll if pushed?\\      1. select(sub=objects)\\      2. filter(condition=that wont roll if pushed; sub=\#1)\\      3. project(projection=shape of \#REF; sub=\#2)\end{tabular}                                                                                                                                                                                                                                                                                                                                                                                                                                                                                                                                                                                                                                                                                                                                                     & \begin{tabular}[c]{@{}l@{}}CopyNet\\      1. select(sub=objects)\\      2. filter(condition=that has roll if pushed; sub=\#1)\\      3. project(projection=shape of \#REF; sub=\#2)\end{tabular}                                                                                                                                                                                                                                                                                                                                                                                                                                                                                                                                                                                                                                                                                          \\ \hline
Additional Steps      & \begin{tabular}[c]{@{}l@{}}What is   the smallestt shape and also yellow?\\      1. select(sub=shapes)\\      2. project(projection=size of \#REF; sub=\#1)\\      3. superlative{[}min{]}(attribute=\#2; sub=\#1)\\      4. filter(condition=that are yellow; sub=\#3)\end{tabular}                                                                                                                                                                                                                                                                                                                                                                                                                                                                                                                                                                                                                                                                                                                    & \begin{tabular}[c]{@{}l@{}}BiaffineGP\\      1. select(sub=shape)\\      2. comparative(condition=smallestt; sub=\#1)\\      3. project(projection=size; sub=\#1)\\      4. superlative{[}min{]}(attribute=\#3; sub=\#1)\\      5. filter(condition=yellow; sub=\#2,\#4)\end{tabular}                                                                                                                                                                                                                                                                                                                                                                                                                                                                                                                                                                                                     \\ \hline
Additional Steps      & \begin{tabular}[c]{@{}l@{}}If at   least five orange dogs without collars sit upright in a row, gazing intently,   in one image, and the other image includes dogs in collars arranged more or   less in a row.\\      1. select(sub=one image)\\      2. project(projection=dogs in \#REF; sub=\#1)\\      3. filter(condition=that are orange; sub=\#2)\\      4. select(sub=collars)\\      5. filter(condition=\#4,without; sub=\#3)\\      6. filter(condition=that sit upright; sub=\#5)\\      7. filter(condition=in a row; sub=\#6)\\      8. filter(condition=that are gazing intently; sub=\#7)\\      9. aggregate{[}count{]}(arg=\#8)\\      10. boolean(condition=is at least five; sub=\#9)\\      11. select(sub=the other image)\\      12. project(projection=dogs in \#REF; sub=\#11)\\      13. filter(condition=\#4,in; sub=\#12)\\      14. boolean(condition=are arranged more or less in a row; sub=\#13)\\      15. boolean{[}logical\_and,true{]}(sub=\#10,\#14)\end{tabular} & \begin{tabular}[c]{@{}l@{}}Latent-RAT\\      1. select(sub=one image)\\      2. project(projection=dogs in \#REF; sub=\#1)\\      3. filter(condition=that are orange; sub=\#2)\\      4. select(sub=collars)\\      5. filter(condition=that are orange; sub=\#3)\\      6. filter(condition=that are in a row; sub=\#5)\\      7. filter(condition=that are gazing intently; sub=\#6)\\      8. aggregate{[}count{]}(arg=\#7)\\      9. boolean(condition=is at least five; sub=\#8)\\      10. select(sub=other image)\\      11. project(projection=dogs in \#REF; sub=\#10)\\      12. project(projection=collars of \#REF; sub=\#10)\\      13. filter(condition=that are arranged more in a row; sub=\#12)\\      14. aggregate{[}count{]}(arg=\#13)\\      15. boolean(condition=is at least five; sub=\#14)\\      16. boolean{[}logical\_and,true{]}(sub=\#8,\#15)\end{tabular} \\ \hline
Wrong Logic           & \begin{tabular}[c]{@{}l@{}}How many   was the difference beween Sobieski's force and the Turks and Tatars?\\      1. select(sub=Sobieski)\\      2. project(projection=the force of \#REF; sub=\#1)\\      3. project(projection=size of \#REF; sub=\#2)\\      4. select(sub=the Turks and Tatars)\\      5. project(projection=the force of \#REF; sub=\#4)\\      6. project(projection=size of \#REF; sub=\#5)\\      7. arithmetic{[}difference{]}(left=\#6; right=\#3)\end{tabular}                                                                                                                                                                                                                                                                                                                                                                                                                                                                                                               & \begin{tabular}[c]{@{}l@{}}Latent-RAT\\      1. select(sub=Sobieski)\\      2. project(projection=force of \#REF; sub=\#1)\\      3. select(sub=Turks)\\      4. select(sub=the Tatars)\\      5. arithmetic{[}difference{]}(left=\#2; right=\#3)\\      6. arithmetic{[}difference{]}(left=\#4; right=\#5)\end{tabular}                                                                                                                                                                                                                                                                                                                                                                                                                                                                                                                                                                  \\ \hline
Wrong Step Structure  & \begin{tabular}[c]{@{}l@{}}How many   years after Knopf was founded was it officiaully incorporated?\\      1. select(sub=Knopf was founded)\\      2. select(sub=Knopf was officiaully incorporated)\\      3. project(projection=year of \#REF; sub=\#1)\\      4. project(projection=year of \#REF; sub=\#2)\\      5. arithmetic{[}difference{]}(left=\#4; right=\#3)\end{tabular}                                                                                                                                                                                                                                                                                                                                                                                                                                                                                                                                                                                                                  & \begin{tabular}[c]{@{}l@{}}BiaffineGP\\      1. project(projection=Knopf was founded years; sub=\#1)\\      2. select(sub=was it officiaully incorporated)\\      3. project(projection=years; sub=\#2)\\      4. arithmetic{[}difference{]}(left=\#3; right=\#1)\end{tabular}                                                                                                                                                                                                                                                                                                                                                                                                                                                                                                                                                                                                            \\ \hline
Out of Vocab          & \begin{tabular}[c]{@{}l@{}}What   coutry is currently led by an acting prime minister and is a part of   NATO?\\      1. select(sub=NATO)\\      2. project(projection=coutries of \#REF; sub=\#1)\\      3. filter(condition=that are currently led by an acting prime minister;   sub=\#2)\end{tabular}                                                                                                                                                                                                                                                                                                                                                                                                                                                                                                                                                                                                                                                                                               & \begin{tabular}[c]{@{}l@{}}CopyNet\\      1. select(sub=company)\\      2. filter(condition=that is currently led by an acting prime minister;   sub=\#1)\\      3. filter(condition=that is part of NATO; sub=\#2)\end{tabular}                                                                                                                                                                                                                                                                                                                                                                                                                                                                                                                                                                                                                                                          \\ \hline
% \end{tabular}
\caption{
Error Classes Examples}
\label{tab:error-analysis-examples}
\end{longtable}
