# Supplementary material for: Question Decomposition with Dependency Graphs
Source: arXiv:2104.08647 source file (2021-04-17)
Supplement: Supplementary file 2 [file graph_creation-tokens_alignment.tex]

\subsection{ILP Based Token Alignment}
\label{sec:ILP-token-alignment}

Recall we denote by $q=\langle q_1, \dots ,q_n \rangle$ the question tokens and by $\forall i\in[1..m], s^i=s^i_1 \dots s^i_{n_i}$  the $i$th step tokens.  An \emph{alignment} is defined by $M=\{(q_i,s^k_j)\mid  q_i\approx s^k_j ;i\in[1..n], k\in[1..m], j\in[1..n_k] \}$, where by $t\approx t'$ we mean $t, t'$ are BREAK-equivalent (see Table \ref{tab:break-equivalance}). We say $t \sim_M t'$ iff $(t,t')\in M$ and $t_{1,\dots,d}\sim_M t_{1,\dots,d}$ iff $\forall i\in[1..d]: t_i\sim_M t'_i$. For readability we mostly omit the $M$ and just write $t \sim t'$ or $t_{1,\dots,d}\sim t'_{1,\dots,d}$ to mark that two tokens/sequences are aligned.

We can formalize the desired alignment restrictions (\S\ref{sec:graph-creation:tokens-alignment}) as an Integer Linear Program. For $i\in[1..n], k\in[1..m], j\in[1..n_k]$ let $x^k_{ij}\in\{0,1\}$ be an indicator for whether $(q_i,s^k_j)$ is in the output alignment, i.e $x^k_{ij} := \mathbbm{1}[(q_i,s^k_j)\in M]$. An assignment for these $\{x^k_{ij}\}$ binary variables defines a possible alignment.
\begin{equation}
    \forall i,j,k: x^k_{ij}\geq 0
\end{equation}
\begin{equation}
    \forall i,j,k: x^k_{ij}\leq 1
\end{equation}
\\

\paragraph{Validity} 
A valid alignment should align only equivalent tokens. Therefor, $x^k_{ij}$ can be $1$ just if $q_i \approx s^k_j$, otherwise it must be $0$. Let $a^k_{ij}\in\{0,1\}:=\mathbbm{1}[q_i \approx s^k_j]$ be an indicator for potential \emph{alignment}. We want to make sure that $a^k_{ij}=0 \Rightarrow x^k_{ij}=0$, so we restrict:
\begin{equation}
    \forall i,j,k: x^k_{ij}\leq a^k_{ij}
\end{equation}
\\

\paragraph{Exact Match} 
Similar to validity section, we define $b^k_{ij}\in\{0,1\}:=\mathbbm{1}[q_i = s^k_j]$ and would like to maximize:
\begin{equation}
    \max\sum_{k,i,j}b^{k}_{ij}x^{k}_{ij}
\end{equation}
\\

\paragraph{Steps Coverage} 
We would like each step token that has some potential question tokens to be aligned to at least one of them, i.e $\forall k,j: \lor_{i=1}^{n}a^k_{ij}\Rightarrow \lor_{i=1}^{n}x^k_{ij}$. Thus, we restrict
\begin{equation}
    \forall k,j: -\sum_{i=1}^{n}a^k_{ij} + n\sum_{i=1}^{n}x^k_{ij} \geq 0
\end{equation}
\\

\paragraph{Sequential Preference} 
We define auxiliary variables to maximize the length of aligned sequences. Let $y^{k,d}_{i,j}\in\{0,1\}, d\in\mathbbm{N}^+$ be an indicator for alignment of a sequence of length $d+1$ starting at $q_i, s^k_j$, i.e $y^{k,d}_{ij}:=\mathbbm{1}[q_{i,\dots,i+d} \sim s^k_{j,\dots,j+d}]$. Note $y^{k,d}_{ij} \iff \land_{p=0}^{d}x^k_{i+p,j+p} $, so we require:
\begin{equation}
    \forall d,k,i,j: -(d+1)y^{k,d}_{ij} + \sum_{p=0}^{d}x^k_{i+p, j+p} \geq 0
\end{equation}
\begin{equation}
    \forall d,k,i,j: y^{k,d}_{ij} - \sum_{p=0}^{d}x^k_{i+p, j+p} \geq -d
\end{equation}

We prefer long sequence alignment, meaning $\{y^k_{ij}\}$ with larger $d$'s to be $1$. We could define a monotonic scoring function that increases with $d$, $c(d):\mathbbm{N}^+\rightarrow \mathbbm{R}$ (e.g $c(d):=d$), and maximize $\sum_{d,k,i,j}c(d)y^{k,d}_{ij}$. However, since $y^{k,d}_{ij} \Rightarrow y^{k,d'}_{i'j'} \quad \forall d',i',j'\quad s.t \quad i\leq i', j \leq j', i'+d'\leq i+d, j'+d'\leq j+d$, we express this with:
\begin{equation}
    \max\sum_{d,k,i,j}y^{k,d}_{ij}
\end{equation}
\\

\paragraph{References Relations} 
Let $r^{k,k'}\in\{0,1\}$ indicate if step $k$ refers to step $k'$. We define auxiliaries variables that will help us count consecutive tokens in the question that are aligned to $k,k'$. $z^{+,k,k'}_i \iff (x^k_i \land r^{k,k'} \land x^{k'}_{i+1})$, $z^{-,k,k'}_i \iff (x^k_i \land r^{k,k'} \land x^{k'}_{i-1})$, where $x^k_i:= \lor_{j=1}^{n_k}x^k_{ij}$ (token $q_i$ is aligned to some token(s) of step $k$). We would like to maximize on $\{z^{+,k,k'},z^{-,k,k'}\}$:
\begin{equation}
    \forall k,i: -x^k_i+\sum_{j=1}^{n_k}x^k_{ij}\geq 0
\end{equation}
\begin{equation}
    \forall k,i: n_kx^k_i-\sum_{j=1}^{n_k}x^k_{ij}\geq 0
\end{equation}
\begin{equation}
    \forall k,k',i: -3z^{\pm,k,k'}_{i} + x^{k}_i + r^{k,k'} + x^{k'}_{i\pm1} \geq 0
\end{equation}
\begin{equation}
    \forall k,k',i: z^{\pm ,k,k'}_{i} - x^{k}_i - r^{k,k'} - x^{k'}_{i \pm 1} \geq -2
\end{equation}
\begin{equation}
    \max\sum_{k,k',i} z^{+ ,k,k'}_{i}+z^{- ,k,k'}_{i}
\end{equation}
\\

\paragraph{Minimalism} 
We want as few alignments as possible so intuitively we would like:
\begin{equation}
    \min\sum_{k,i,j}x^{k}_{ij}
\end{equation}
However, this constraint is not enough when there is a repeated question token/phrase that is aligned to more than one step. We would like each of the steps to be aligned to a separate copy of that phrase, i.e, each question token should be aligned to as few steps as possible, and ideally to a single \emph{unique} step. Let $u^{d}_{i}$ be an indicator for $q_i$ being aligned to at most $d \in \mathbbm{N}^+$ different steps, i.e, $u^d_i:=\mathbbm{1}(\exists K \subseteq [1..m], |K|\geq d: \forall k \in K, x^k_i=true)$. Intuitively, we want as few as possible such $u$'s for large $d$'s to be true. Since $\forall d,d', d \leq d' : u^{d'}_i \Rightarrow u^d_i$, it is enough to minimize over these $u$'s.
\begin{equation}
    \forall i,d: -du^d_i+\sum_{k}x^{k}_{i} \geq 0
\end{equation}
\begin{equation}
    \forall i,d: -mu^d_i + \sum_kx^k_i \leq d-1
\end{equation}
\begin{equation}
    \min\sum_{i,d}u^{d}_{i}
\end{equation}
\\

Eventually, our objective function is:\\
$
    \min\biggl[
    c_{min} \sum_{k,i,j}x^{k}_{ij} \\
    +c_{unique} \sum_{i,d}u^{d}_{i} \\
    -c_{exact} \sum_{k,i,j}b^{k}_{ij}x^{k}_{ij} \\
    -c_{seq} \sum_{d,k,i,j}y^{k,d}_{ij} \\
    -c_{ref} \sum_{k,k',i} (z^{+ ,k,k'}_{i}+z^{- ,k,k'}_{i})
    \biggr]
$ \\
Where we are taking $c_{min} \gg c_{unique} \gg c_{seq} \gg c_{exact}, c_{ref} $ to express the priorities between the preferences.
