# Supplementary material for: Question Decomposition with Dependency Graphs
Source: arXiv:2104.08647 source file (2021-04-17)
Supplement: Supplementary file 3 [file graph_decoding.tex]

\subsection{Dependency Graph Decoding}
\label{sec:gependencies-graph-decoding}
Our graph parser predicts probabilities over possible assignment of tags for every possible arc on top of the given tokens, but is not aware of any structural constraints during learning. We use a soft conversion into SDG in favor of evaluation and also provide an ILP-based post processing for fixing the produced probabilities according to the structural constraints.

\subsubsection{Soft Decoding}
Given a predicted DG we softly convert it into a SDG by first grouping the tokens into spans with respect to the \emph{span} dependencies. Two tokens are considered in the same span if there is an undirected path of \emph{span} dependencies between them. Doing so we allow no left-to-right \emph{span} dependencies, and multiple in/out \emph{span} dependencies to/from a single token. The dependencies between spans are induced by projecting their members' dependencies.
\subsubsection{ILP Based Decoding}
We formalize the DG specification to ILP constraints and solve an ILP with respect to the predicted probabilities.

Let $\mathcal{P} = \{p(i,j,t)\}$ be the predicted probabilities of a graph parser, where $\forall i,j \in [n], t \in Tags \cup \{none\}: p(i,j,t):=P[\textrm{the tag of arc (i,j) is t}]$. We would like to find a valid graph $G$ with maximal probability under $\mathcal{P}$ among the valid graphs. 

Denote $T := Tags$, $\bar{T} := T \cup \{none\}$. Let $x_{i,j,t}\in\{0,1\}$ be our target variables, i.e, $\forall i \in [n], j \in [n], t\in T,\ x_{i,j,t} := \mathbbm{1}[\textrm{the tag of arc (i,j) is t}]$. Note we omit $\{x_{i,j,none}\}$ to reduce the amount of variables, since $x_{i,j,none} = 1 - \sum_{t \in T}{x_{i,j,t}}$.

\paragraph{Maximal Probability} 
We would like our graph to maximize the probabilities given by $\mathcal{P}$, so our objective has to maximize:
\begin{equation}
\begin{split}
& \max \prod_{i,j;t\in \bar{T}} x_{i,j,t} p(i,j,t) = \\
& \max \sum_{i,j;t\in \bar{T}} x_{i,j,t} \log{p(i,j,t)} = \\
& \max \sum_{i,j;t\in T} x_{i,j,t} \log{p(i,j,t)} + \\ & \sum_{i,j} \left( 1- \sum_{t\in T}x_{i,j,t} \right) \log{\left( 1- \sum_{t\in T}p(i,j,t) \right)}
\end{split}
\end{equation}

\paragraph{Single Tag} 
We allow each arc to have a single tag only (or \emph{none}).
\begin{equation}
\forall i,j: \ \sum_{t\in T} x_{i,j,t} \leq 1
\end{equation}

\paragraph{Valid No-Operational Dependencies} 
\emph{span} and \emph{duplicate} have a specific roll which can be valid regardless of the other choices. \emph{span} is left-to-right, and \emph{duplicate} is from a \emph{[DUP]} token to a no-auxiliary token (\emph{[RSC], [DUP], [DUM]}). Let $a_{i,j,t} \in \{0,1\}$ be indicators for allowed tagging. We demand
\begin{equation}
\forall i,j,t \in T \ x_{i,j,t} \leq a_{i,j,t}
\end{equation}
And define $a_{i,j,t}$ to be $1$ except for the following cases
\begin{equation}
\forall i \geq j \ a_{i,j,span}=0
\end{equation}
\begin{multline}
\forall i,j: q_{i} \neq \text{[DUP]} \lor q_{j} \in \{\text{[RSC],[DUP],[DUM]}\} \\ \Rightarrow a_{i,j,duplicate}=0
\end{multline}
Moreover, each node can have at most a single incoming (outgoing) \emph{span} dependency, and at most a single outgoing \emph{duplicate}:
\begin{multline}
\forall i: \sum_{j} x_{i,j,span} \leq 1 \\ 
\forall j: \sum_{i} x_{i,j,span} \leq 1 \\
\forall i: \sum_{j} x_{i,j,duplicate} \leq 1 \\
\end{multline}
And finally, \emph{[DUP]} with some incoming/outgoing arcs must have an outgoing \emph{duplicate}, i.e, $\lor_{j, t}(x_{i,j,t} \lor x_{j,i,t}) \Rightarrow \lor_{j}x_{i,j,duplicate}$.
\begin{multline}
    \forall i, q_i=[DUP]: \\ -\sum\limits_{j,t}(x_{i,j,t}+x_{j,i,t})+2n|T|\sum\limits_{j}x_{i,j,duplicate} \geq 0
\end{multline}

\paragraph{Consistent Dependencies} 
Recall dependencies (tags) are given by triplets of the form $\langle operator, properties, arg \rangle$ (e.g $\text{filter-sub[equals]} = \langle filter, [equals], sub \rangle$). Since the outgoing arcs define a node operation we would like them to be consistent, i.e have the same \emph{operator} and \emph{properties}.

Let $\mathcal{O}$ be the possible operations and $Op:T \rightarrow \mathcal{O}$ a mapping from each tag (besides \emph{none}) to its operation. We define auxiliary variables $y_{i,o}^{out} \in \{0,1\}$ to indicates there is an outgoing arc from node $i$ with an operation $o$, and demand
\begin{equation}
\forall i  \ \sum_{o \neq duplicate} y_{i,o}^{out} \leq 1
\end{equation} 
More formally, $y_{i,o}^{out} := \mathbbm{1} \left[ \exists j \in [n], t \in T: x_{i,j,t}  \land Op(t)=o \right]$, and therefore $y_{i,o}^{out} = 1 \Leftrightarrow \sum_{j,t}x_{i,j,t}\mathbbm{1}\left[ Op(t)=o \right] \geq 1$. We obtain this by
\begin{multline}
\forall i, o \neq duplicate: \\ -\sum_{j,t}x_{i,j,t}\mathbbm{I}\left[ Op(t)=o \right] + n |T|y_{i,o}^{out} \geq 0
\end{multline} 
\begin{multline}
\forall i, o \neq duplicate:  \\ -y_{i,o}^{out} + \sum_{j,t}x_{i,j,t}\mathbbm{I}\left[ Op(t)=o \right] \geq 0
\end{multline} 

\paragraph{Span Single Representative} 
Recall a span is a left-to-right chain of \emph{span} arcs, where the rightmost token is used as the span representative. Each arc in/from this span should use the representative only. To achieve this, for each $j$ which is a non-representative node in a span chain, i.e, $y_{j,span}^{out} = 1$, we demand that $j$ will not have any incoming arcs but (maybe) a single \emph{span}, i.e $ \sum_{i,t\in T\setminus\{span\}}x_{i,j,t} \leq 0$ and $ \sum_{i}x_{i,j,span} \leq 1$.
\begin{multline}
\forall j:\\  \sum_{i,t\in T\setminus\{span\}}x_{i,j,t} + n(|T|-1)y_{j,span}^{out} \leq n(|T|-1)
\end{multline}
\begin{equation}
\forall j:  \sum_{i}x_{i,j,span} + ny_{j,span}^{out} \leq n + 1
\end{equation} 

\paragraph{Valid Dependency Combination} 
Operations sometimes induces constraints on dependency combinations. For example, \emph{union} must have at least two subjects; \emph{arithmetic-left} should be combined with \emph{arithmetic-right}, etc. Note that an argument might be ``missing'' (no outgoing dependency, no reference) if it's corresponding information is embedded in the span itself (e.g \emph{arithmetic[diff](left=\#1, right="100")}). If so, given a set of desired arguments we demand each of them has a corresponding arc pointing to a non-empty span, except (maybe) one if the current span is not empty.

We start by defining indicators for non-empty spans. First, mark no-empty tokens (s.a \emph{the, a, that, [RSC], [DUP], [DUM]}) using $m_{i}\in \{0,1\}$. Next, define $c_{i} \in \{0,1\}$ to be indicators for $q_{i}$ be a part of a content-holder (no-empty) span. We define $c_{i}$ in a recursive manner by $c_{i} \coloneqq m_i \lor \left( \lor_{k<i}(x_{k,i,span}\land c_{k}) \right) $ and if $q_i = \text{[DUP]}$ we add $\lor_{k<i}x_{i,k,duplicate}m_k$.

We add auxiliary variables $c_{k,i}:=x_{k,i,span} \land c_{k}$ and demand:
\begin{equation}
\begin{split}
\forall k \leq i: \\
2c_{k,i}-(x_{k,i,span}+c_k) \leq 0 \\
-c_{k,i}+(x_{k,i,span}+c_k) \leq 1
\end{split}
\end{equation}
\begin{equation}
\begin{split}
\forall i, q_i \neq \text{[DUP]}: \\
c_{0} := m_{0} \\
\sum_{k<i}c_{k,i}+m_{i}+(1-c_{i}) \geq 1 \\
-(\sum_{k<i}c_{k,i}+m_{i})+ic_{i} \geq 0
\end{split}
\end{equation}
\begin{equation}
\begin{split}
\forall i, q_i = \text{[DUP]}: \\
\sum_{k<i}c_{k,i}+\sum_{k<i}x_{i,k,dup}m_k+m_{i}+(1-c_{i}) \geq 1 \\
-(\sum_{k<i}c_{k,i}+\sum_{k<i}x_{i,k,dup}m_k+m_{i})+ic_{i} \geq 0
\end{split}
\end{equation}
Now, if we want a specific combination, $\tau=t_1, \dots , t_{|\tau|} \subseteq T$ to take place together (or not at all) we can demand $\sum_{t\in\tau}\bar{y}_{i,t}^{out}+c_i \geq |\tau|$ or $\sum_{t\in\tau}\bar{y}_{i,t}^{out} \leq 0$, where $\bar{y}^{out}_{i,t}$ are defined as $y^{out}_{i,o}$, but for full tags instead of just the operations. Let $z^{+}_{i,\tau}$, $z^{-}_{i,\tau}$ be indicators for these two conditions respectively. We want $z^{+}_{i,\tau} \lor z^{-}_{i,\tau}$ to hold.
\begin{equation}
\begin{split}
\forall i, \tau: \\
-|\tau|z^{-}_{i,\tau} + \sum_{t\in\tau}(1-\bar{y}^{out}_{i,t}) \geq |\tau| \\
-\sum_{t\in\tau}(1-\bar{y}^{out}_{i,t})+|\tau|z^{-}_{i,\tau} \geq 1-|\tau|
\end{split}
\end{equation}

\begin{equation}
\begin{split}
\forall i, \tau: \\
|\tau|(1-z^{+}_{i,\tau}) + \sum_{t\in\tau}\bar{y}^{out}_{i,t_h}+c_i \geq |\tau| \\
-2z^{+}_{i,\tau} +
\sum_{t\in\tau}\bar{y}^{out}_{i,t_h}+c_i < |\tau|
\end{split}
\end{equation}

\begin{equation}
    \forall i, \tau: z^{+}_{i,\tau} + z^{-}_{i,\tau} = 1
\end{equation}

Additional form of valid combinations constraint is $<\tau,\tau_{trigger}>$ where $\tau_{trigger} \subseteq \tau$ are dependencies that imply $\tau$, i.e, if one of $t_{i}, i \in \tau_{trigger}$, holds we want the entire $\tau$ to hold.

\paragraph{Connectivity}
Each QDMR step should be referred by other steps, except for the last step. Therefore, only a single span can have no incoming dependencies, i.e, be a \emph{root}. A \emph{root} (1) should have an outgoing dependency; (2) be a representative of a span (no outgoing \emph{span} dependency); (3) have no incoming dependency. 

Let $\{r_i\}_{i=1}^{n}$ be indicators for $q_i$ be a \emph{root}. We want $r_i \Leftrightarrow (1) \bigvee \limits_{j,t} x_{i,j,t} \lor \bigvee \limits_{k}x_{k,i,span}$ and $(2) \bigwedge \limits_{j} \lnot x_{i,j,span}$ and $(3) \bigwedge \limits_{k, t\neq span}\lnot x_{k,i,t}$, i.e $r_i=1 \Leftrightarrow \sum_{j,t}x_{i,j,t} + \sum_{k}x_{k,i,span} \geq 1 \land \sum_{k,t\neq span}x_{k,i,t} + \sum_{j}x_{i,j,span} \leq 0$. We demand
\begin{equation}
\begin{split}
    -r'_i + \sum_{j,t}x_{i,j,t} + \sum_{k}x_{k,i,span} \geq 0 \\
    -\sum_{j,t}x_{i,j,t} -\sum_{k}x_{k,i,span} + n(|T|+1)r'_i \geq 0
\end{split}
\end{equation}
\begin{equation}
\begin{split}
    -(1-r''_i) + \sum_{k,t\neq span}x_{k,i,t} + \sum_{j}x_{i,j,span} \geq 0 \\
    -\sum_{k,t\neq span}x_{k,i,t} - \sum_{j}x_{i,j,span} + n|T|(1-r''_i) \geq 0
\end{split}
\end{equation}
\begin{equation}
\begin{split}
    -2r_i+r'_i+r''_i \geq 0 \\
    -r'_i -r''_i +r_i \geq -1
\end{split}
\end{equation}
Finally we allow at most a single root
\begin{equation}
    \sum_{i}r_i \leq 1
\end{equation}
