# Supplementary material for: Question Decomposition with Dependency Graphs
Source: arXiv:2104.08647 source file (2021-04-17)
Supplement: Supplementary file 4 [file eval-normalized-em.tex]

\subsection{Rule-Based Evaluation (NormEM)}
\label{sec:eval-rule-based}
\todo{fill}
